# Supplementary material for: S2-Attention: Hardware-Aware Context Sharding Among Attention Heads
Source: arXiv:2407.17678 source file (2025-02-05)
Supplement: Supplementary file 1 [file appendix.tex]

\section*{Appendix A: Model Convergence}
To understand if trainings of different attention patterns converge similarly, we design experiments with dense attention, homogeneous and heterogeneous \ours. Results are shown in Figure \ref{fig:loss}. We observe that the model with heterogeneous \ours has almost identical loss curve as the dense attention one, showing same convergence. On the other hand, the model with homogeneous \ours clearly shows a disadvantage in loss.

\begin{figure}[ht!]
    \centering
    \includegraphics[width=0.42\linewidth]{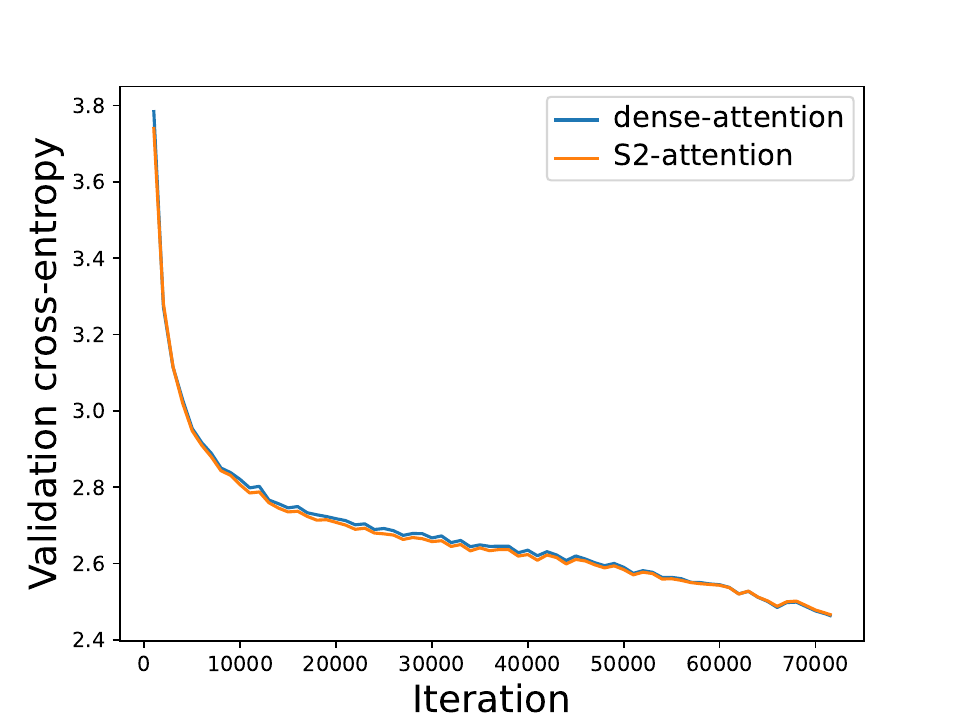}
    \includegraphics[width=0.42\linewidth]{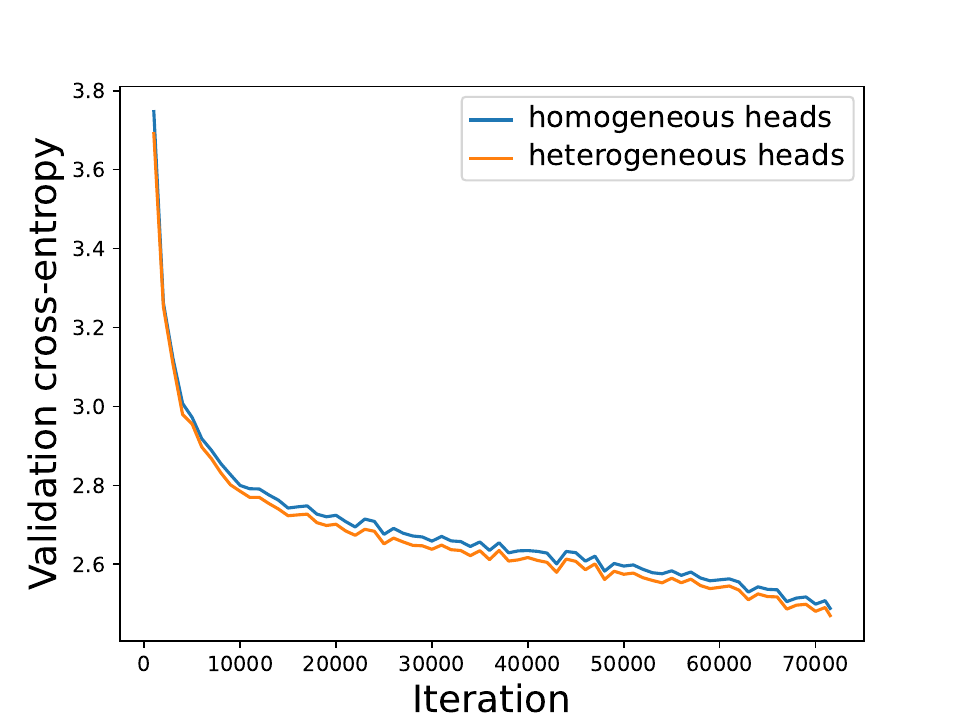}
    \caption{Convergence among dense attention, homogeneous and heterogeneous \ours. \textbf{Left}: dense attention vs heterogeneous\ours. \textbf{Right}: homogeneous vs heterogeneous with complete shards. All experiments are done with identical setting except the attention patters. For \ours, local window = 8,  vertical stride = 16, shard size = 64 tokens.}
    \label{fig:loss}
\end{figure}

\section*{Appendix B: S2-Attention Code Interface}
\label{app:code}
We showcase two examples of using \kernelname to implement customized sparse attention here.
The first chunk of code implements a sparse attention with a dense local window and stride patten outside the window.
Users can make the pattern heterogeneous among attention heads by setting the $homo\_head$ option as False, which will automatically offset the starting index of the stride pattern in each attention head's by the corresponding head index.
Users can specify the granularity of block-sparse mask size by changing the $block\_size$.
GQA and retrieval head can be customized by changing the number of KV heads and number of dense heads respectively.
Lastly, tensor parallel can be enable with the active head range, which is made compatible with the Megatron API.
\begin{figure}[ht!]
    \centering
    \includegraphics[width=0.99\linewidth]{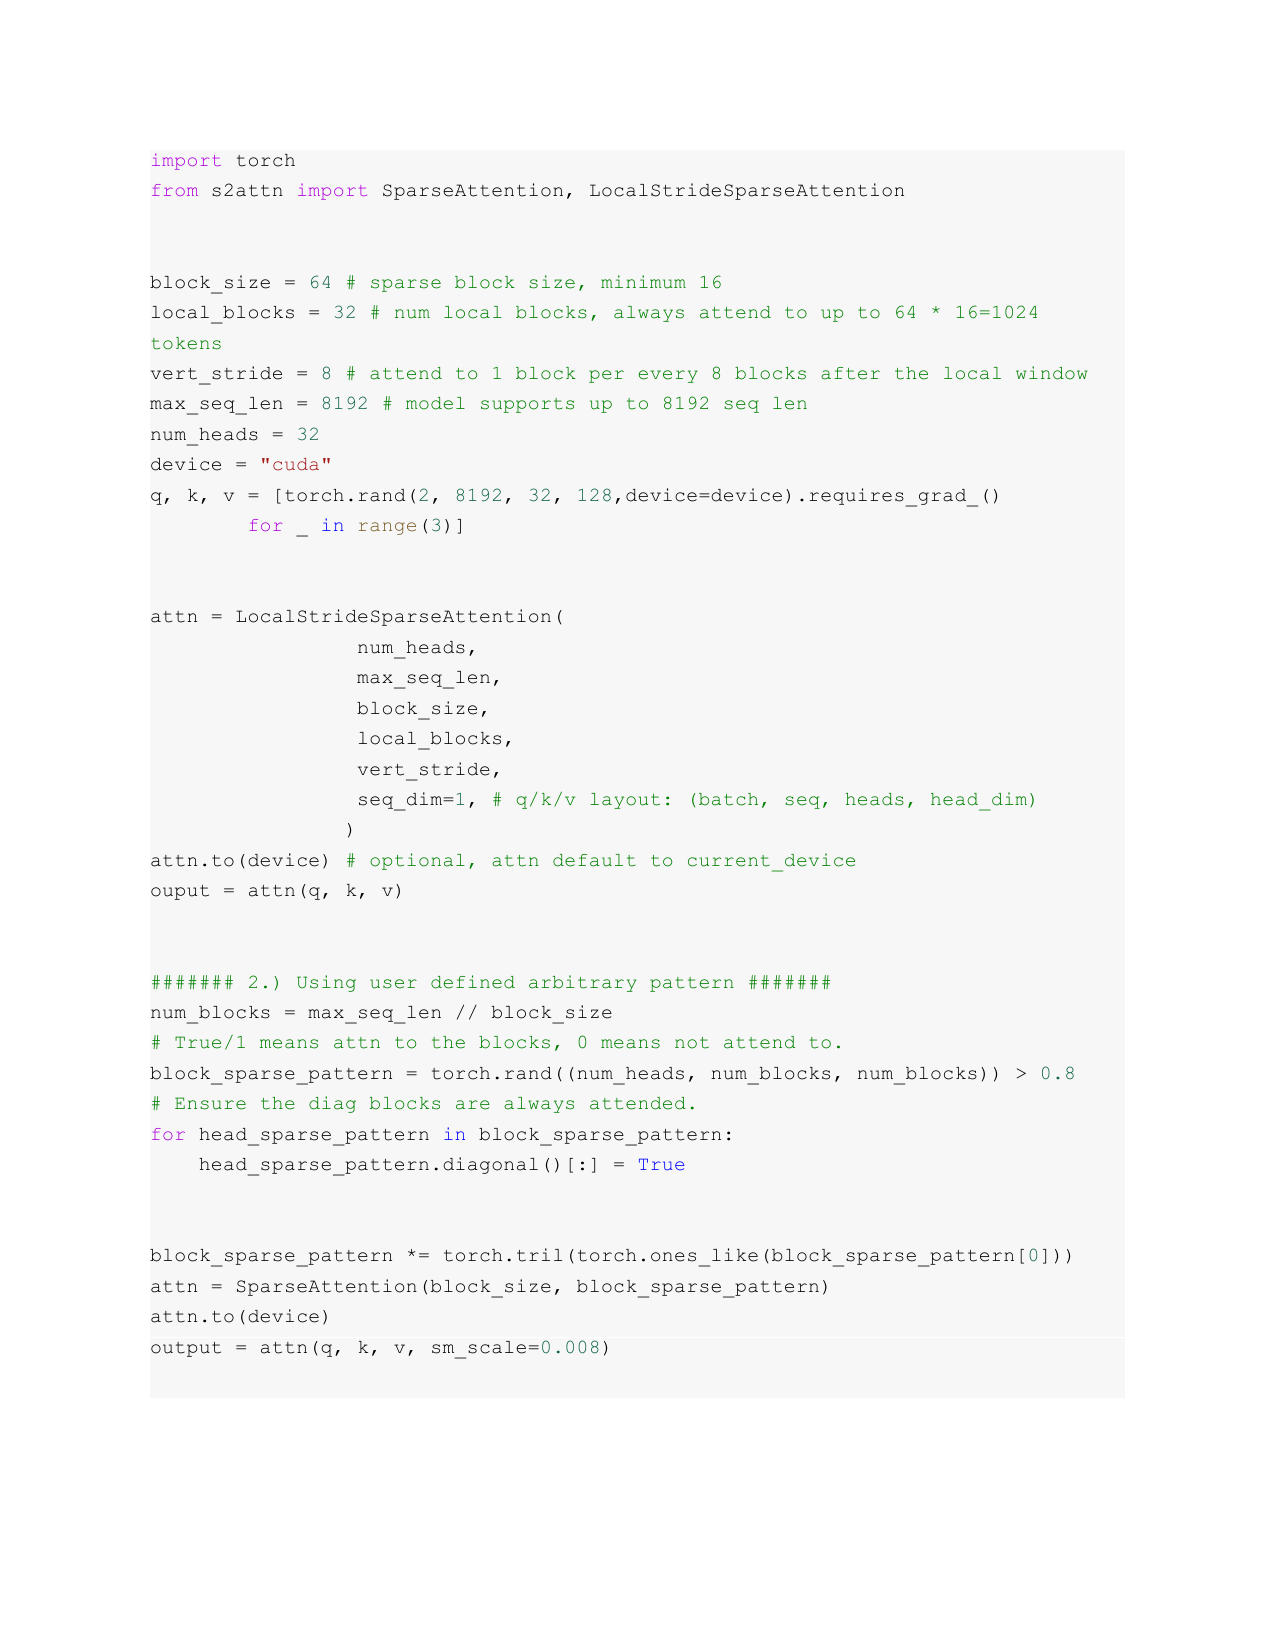}
    \caption{Example usage of S2-Attention.}
    \label{fig:loss}
\end{figure}

\section*{Appendix C: Other Optimizations on the Kernel} 
% Moved to Appendix C
% \hao{suggestion on this one:
% it should focus on what we actually did rather than we didn't do.
% also, i'd use wordings that reflect the insights behind this design choice instead of the current
% empirical wording that "we tried something and this is what worked for us"
% }
Different from FlashAttention, which loads the whole head dimension(D) at once to SRAM, 
we split the QKV vecotrs along head dimension to lower the SRAM usage for each tile.
% \hao{can you fill in this? not sure i'm able to accurately describe this} 
% which is intuitive as the whole vector is needed to compute the attention scores. 
However, in our experiment, we found that split over the D dimension in many cases is beneficial. 
We suspect that this is because Split-D reduce SRAM usage and enable a larger degree of software pipelining. 
Interestingly, we also find that with shard size of 64, Split-D only helps when head dimension is 128, the most commonly used case, while has no additional benefit when head dimension is 64 or 256.
We suspect that this is due to under-tuned hyper-parameters like kernel tile sizes.

\begin{figure}[ht]
  \centering
  \begin{subfigure}[b]{0.24\textwidth}
      \centering
      \includegraphics[width=\textwidth]{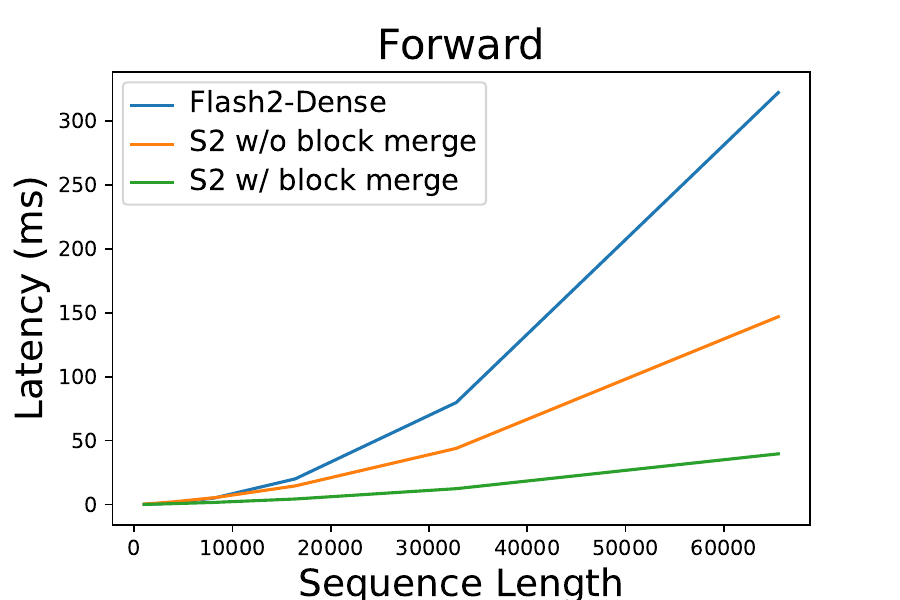}
      \caption{Forward w/ Merge-Q.}
      \label{fig:mergeqfwd}
  \end{subfigure}
  \hfill
  \begin{subfigure}[b]{0.24\textwidth}
      \centering
      \includegraphics[width=\textwidth]{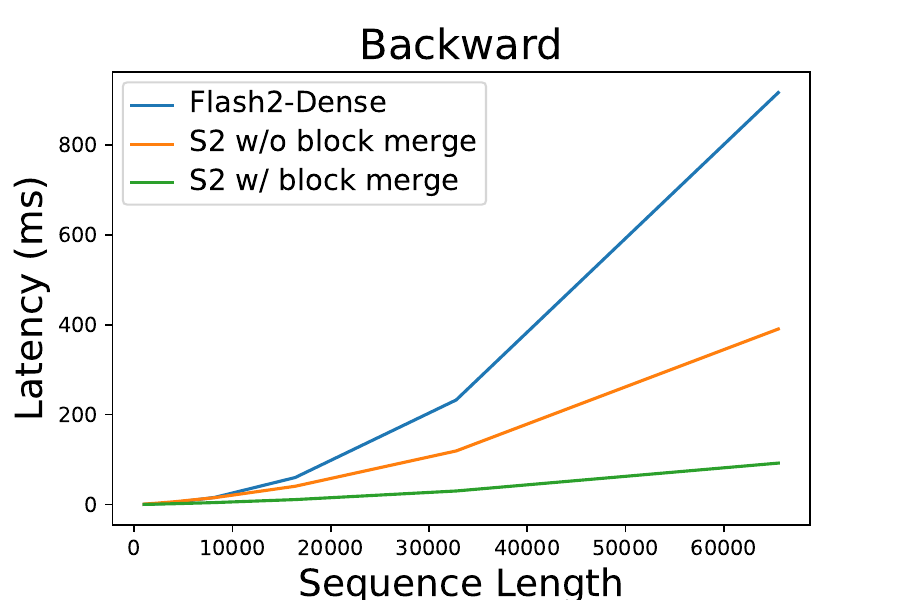}
      \caption{Backward w/ Merge-Q.}
      \label{fig:mergeqbwd}
  \end{subfigure}
  \hfill
  \begin{subfigure}[b]{0.24\textwidth}
      \centering
      \includegraphics[width=\textwidth]{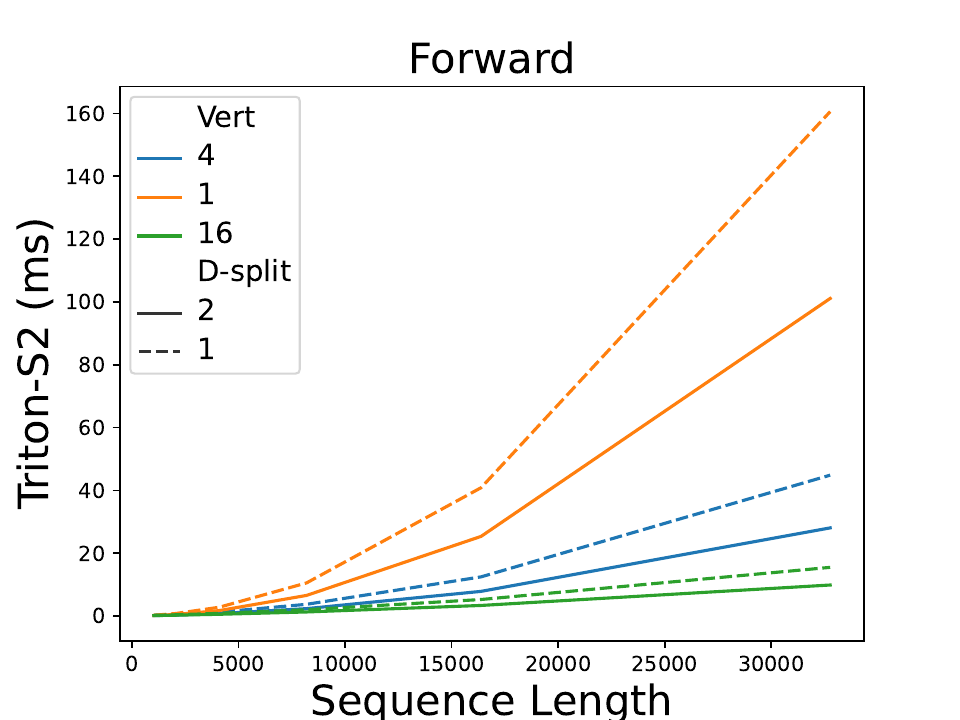}
      \caption{Forward w/ Split-D.}
      \label{fig:dsplitfwd}
  \end{subfigure}
  \hfill
  \begin{subfigure}[b]{0.24\textwidth}
      \centering
      \includegraphics[width=\textwidth]{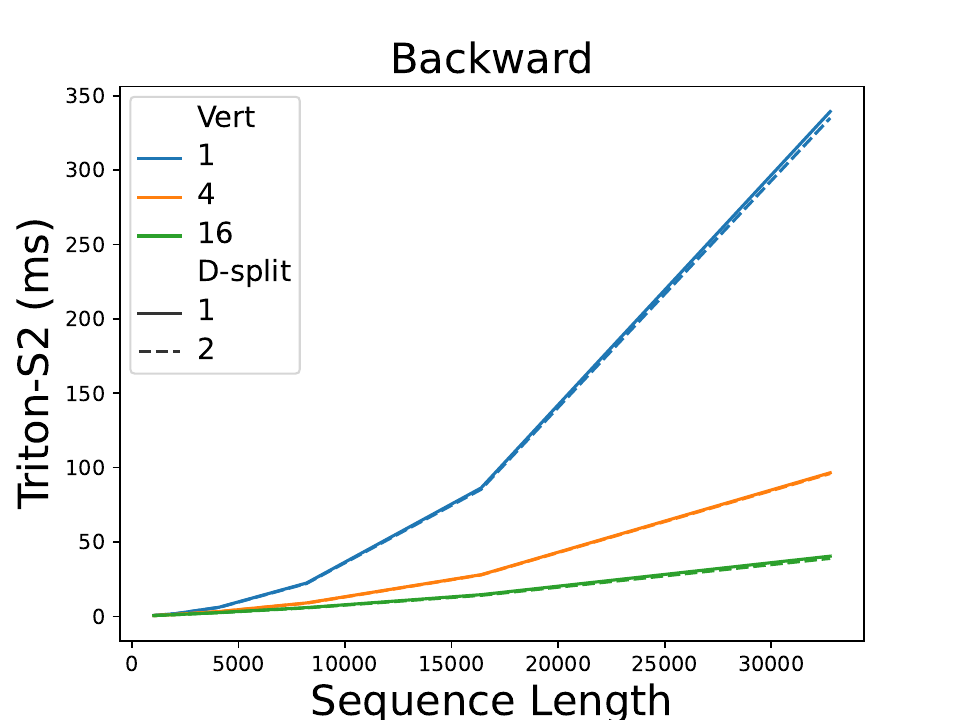}
      \caption{Backward w/ Split-D.}
      \label{fig:dsplitbwd}
  \end{subfigure}
  \caption{Benchmark Latency Improvement with Merge-Q and Split-D.} All experiments are done using (batch, heads, head dim) = (4,
16, 128) on an A100 80GB-SXM GPU. In (a) and (b), (shard size, vertical stride) = (16, 16). In (c) and (d), the shard size is 64.
  \label{fig:trickbenchmark}
\end{figure}

\section*{Appendix D: Implementation Discussion}
For implementation, we twisted the CSR definition to use the data array to store how many times a $kshard[i]$ is used in the mega-shard. 
A merge of $M$ blocks into a single mega block helps reduce the repetition of loading KV shards by $M$ folds in the forward pass and in the backward pass for dQ. As for dK, dV in the backward pass, this does not reduce the loading of Q blocks, but it will reduce the number of times to re-normalize the softmax which utilizes the slower CUDA core instead of TensorCore.
% \textcolor{red}{The possibility to merge K/V blocks are to be explored in the future.}

As shown in Figure \ref{fig:trickbenchmark}, merging multiple small blocks along the Q dimension leads to significant efficiency gains.
For shard sizes larger than the optimal kernel block size, we simply divide them into several smaller shards that are optimal for the GPUs.
